# Supplementary material for: Markov modeling for a satellite tag data record of whale diving behavior
Source: arXiv:2408.09557 source file (2024-08-18)
Supplement: Supplementary file 1 [file supplement.pdf]

# Supplement to "Markov modeling for a satellite tag data record of whale diving behavior"

Joshua Hewitt[1*†], Nicola J. Quick[2,3†], Alan E. Gelfand[1†] and Robert S. Schick[2†]

[1*]Department of Statistical Science, Duke University, Durham, 27708, North Carolina, USA.
[2]Nicholas School of the Environment, Duke University, Durham, 27708, North Carolina, USA.
[3]University of Plymouth, Plymouth, UK.

*Corresponding author(s). E-mail(s): joshua.hewitt@duke.edu; Contributing authors: nicola.quick@duke.edu; alan@duke.edu; robert.schick@duke.edu;
†These authors contributed equally to this work.

## 1 Posterior convergence

We assess convergence of the MCMC sampler visually. Each chain moves from its initial values toward a common region of the parameter space (Figure 1). Each chain locally converges around one of several common values of the parameter space (Figure 2). The convergence behavior suggests the high-dimension parameter space may be multi-modal (when accounting for $\boldsymbol{B}_{ik}$ and $\Sigma_{kn}$), with most of the modes being concentrated around a small region of the parameter space. Few chains converge to values of $\pi_1 > .9$, but we note that there is some evidence for $\pi_1 \approx 1$ as a sensible posterior mode [1].

## 2 Posterior simulation for covariate effects

Posterior predictive simulations used to interpret covariate effects require a sequence $\ell_{01}, \ldots, \ell_{0,12}$ that will initialize recent diving activity covariates for

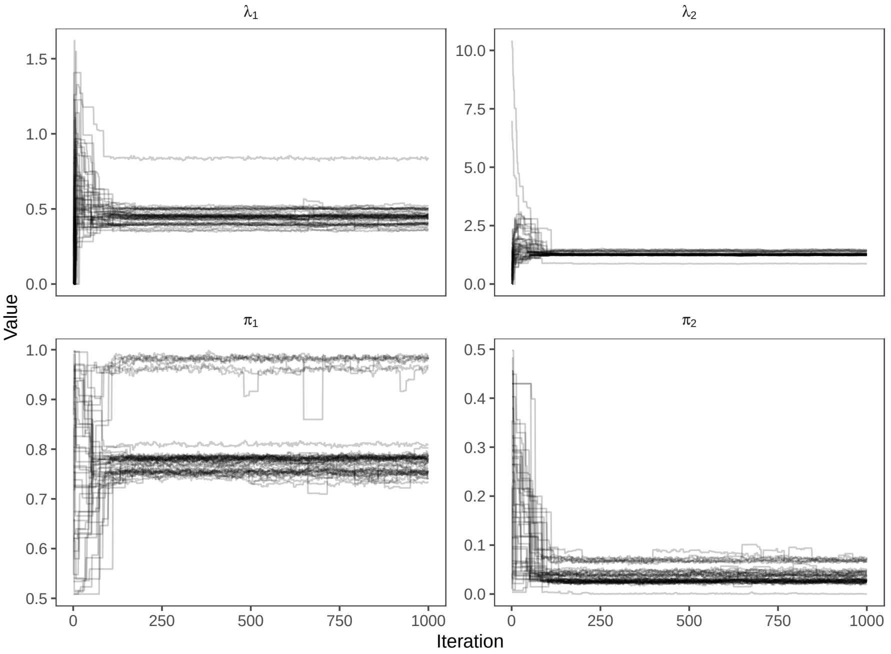


**Fig. 1** First 1,000 iterations of MCMC samplers across independent chains.

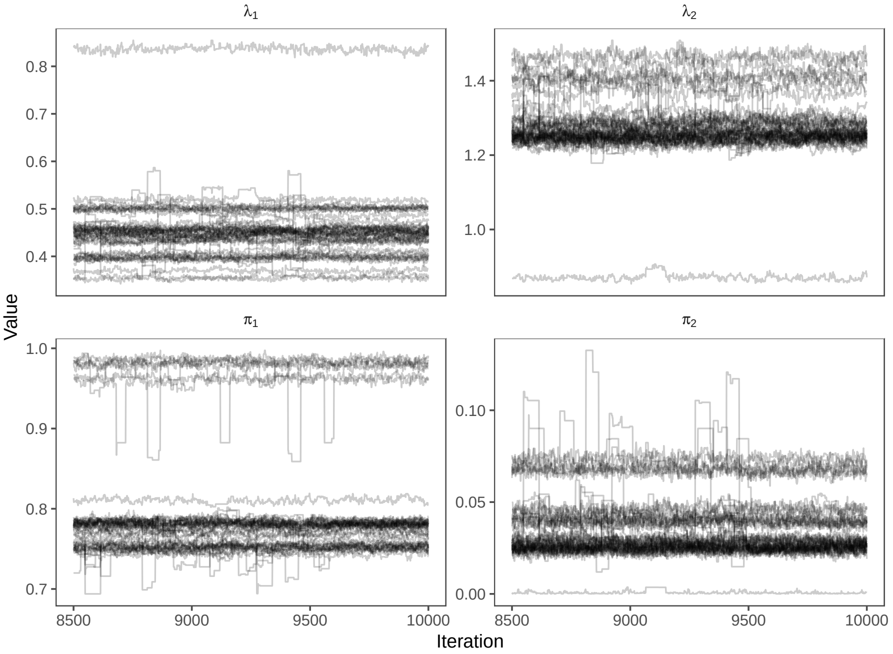


**Fig. 2** Final 1,500 iterations of MCMC samplers across independent chains.

simulation. We use three distinct values for the simulation sequence, which capture the main variability in recent diving activity. The sequences are determined through exploratory clustering to ensure that posterior simulation is initialized from realistic diving behavior.

First, the data are filtered to extract all sequences $\ell_{ij}, \ldots, \ell_{ij+12}$ that end on the surface bin (i.e., such that $\ell_{ij+12} = 1$). The sequences of interest all end at the surface bin because we wish to interpret covariate effects on the first deep-depth hitting time from the surface bin $H_1(1)$. The filtering yields 6,759 sequences of interest.

Then, the sequences of interest are classified into 25 groups via k-means clustering. The k-means algorithm is applied directly to the sequences $\ell_{ij}, \ldots, \ell_{ij+12}$, rather than their transformation to covariates. The number of groups is chosen through exploration with a goal to make the sequences within each cluster reasonably homogeneous, and to make the cluster centers fairly representative of the variability in recent diving activity present in the data (Figure 3).

The cluster centers are used as candidates for the sequence $\ell_{01}, \ldots, \ell_{0,12}$ that will initialize recent diving activity covariates for simulation. Visually, the cluster centers tend to represent 3 main types of recent diving activity: recently finished a deep dive, recovering from deep diving activity, no recent deep diving activity. The additional visual grouping of the k-means cluster centers further suggests 25 clusters offers sufficient data exploration and reduction for initializing posterior simulations. We choose three cluster centers to initialize posterior simulation (see Figure 3 in the manuscript). The recent diving activity covariates at the final timepoint $\boldsymbol{x}_{0,12}$ for the selected clusters spans the range of such values observed among the cluster centers (Figure 4).

Per-animal variability in the posterior predictive distribution for $H_1(1)$ exists due to the random effects (Figure 5).

# References

[1] Hewitt, J., Schick, R.S., Gelfand, A.E.: Continuous-time discrete-state modeling for deep whale dives. Journal of Agricultural, Biological and Environmental Statistics **26**(2), 180–199 (2021). https://doi.org/10.1007/s13253-020-00422-2

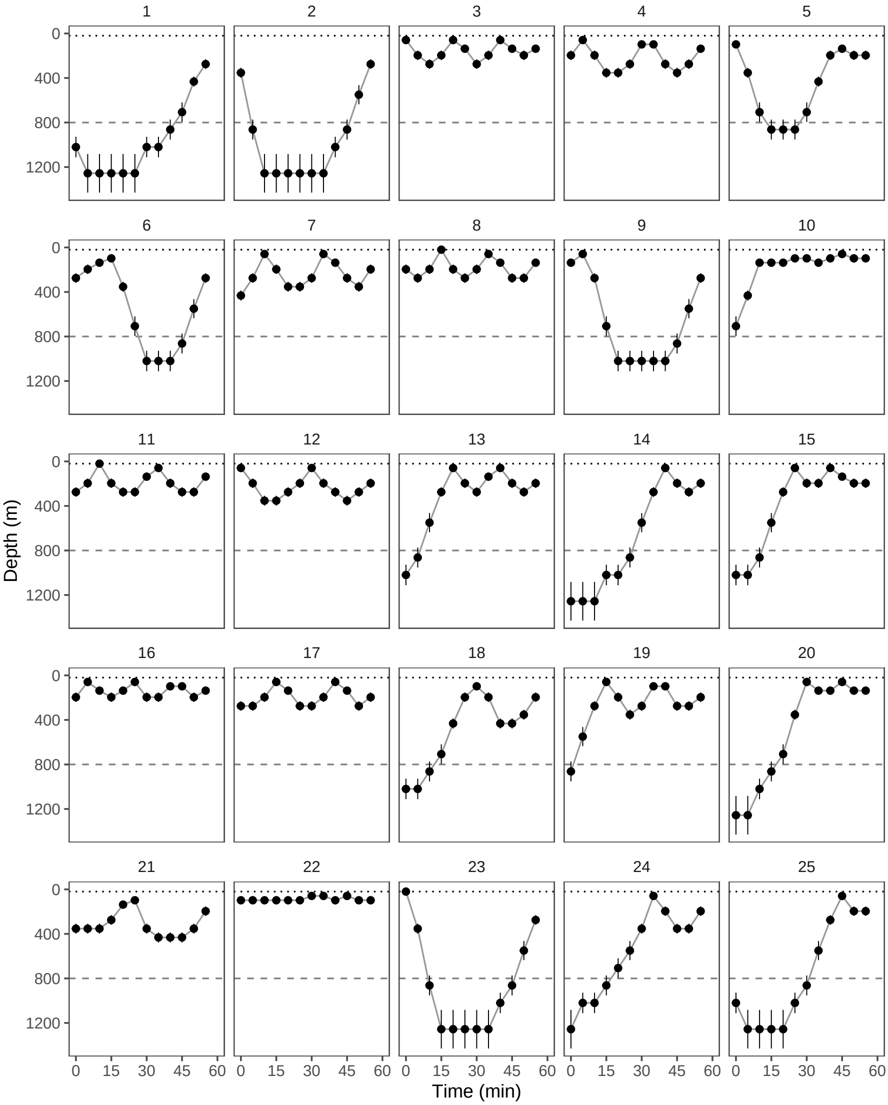


**Fig. 3** Alternate depth bin sequences $\ell_{01}, \ldots, \ell_{0,12}$ that could be used to start posterior simulations for parameter interpretation.

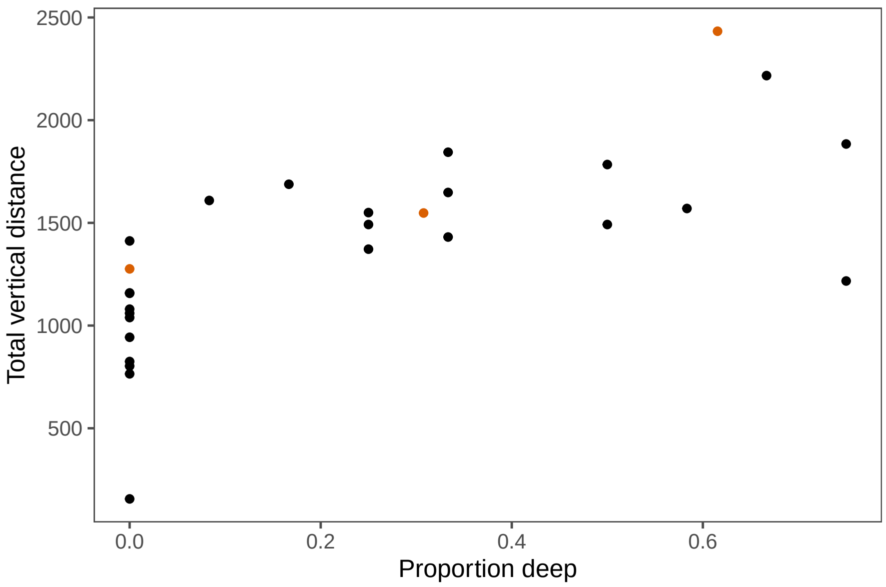


**Fig. 4** Recent diving behavior covariates for dive segments that could be used to start posterior simulations for parameter interpretation. Covariate values for selected dives are highlighted in red.

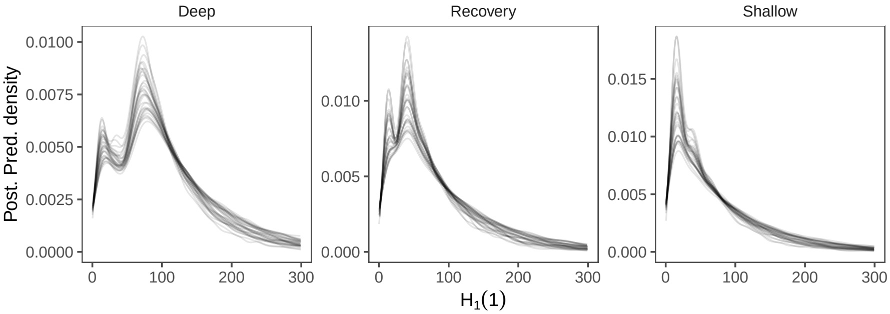


**Fig. 5** Posterior predictive distributions for $H_1(1)$ for each animal, conditional on simulations started from daytime and with an initial fast descent movement. The earlier mode in the distributions is associated with dives that continued the initial fast descent movement, diving deep quickly, while the later mode in the distributions is associated with dives that transitioned out of the initial fast descent movement, taking longer overall to dive deep.
